# Supplementary material for: Dijkstras algorithm with predictions to solve the single-source many-targets shortest-path problem
Source: arXiv:2112.11927 source file (2023-03-04)
Supplement: Supplementary file 1 [file 8_appendix.tex]

% !TEX root = 00_main.tex


\newpage
\appendix


\iffalse

\subparagraph*{Fine-grained Results for Different Algorithms.}
%
We present some more fine-grained results for all algorithms in Table~\ref{tbl:all_results}.
In addition to the basic queue operations stated in Table \ref{tbl:result1}, we also keep track of various other operations. 
The meaning of the labels are as follows: 
$\textit{INR}$ indicates the number of nodes that are inserted into but never removed from the priority queue. 
$\textit{RRM1}$ is the number of nodes that are moved from $R$ to $\pq$ not due to a restart, while 
$\textit{RRM2}$ is the number of nodes that are moved from $R$ to $\pq$ due to a restart (batch insertion). 
$\textit{RIS}$ is the number of nodes added to $R$ and 
$\textit{RDP}$ is the number of times the distance of a node in $R$ is updated. 

The number of nodes that are inserted into but never removed from the queue ($\textit{INR}$) is where one would expect the most savings by our \DijkstraLearning\ algorithms (see also Section \ref{s:lower-bound}). 
The experiments indeed confirm this: our algorithm saves a significant fraction of these operations (both with \smart\ and \naive) compared to \DijkstraPruning\ (which in turn already saves a large fraction of these operations with respect to $\Dijkstra$). 
In the \DijkstraLearning\ with \smart\ algorithm, some extra book-keeping needs to happen in order to perform the restart. For our test set, there are approximately $\sim$46 insertions into $R$ and $\sim$15 moves from a node from $R$ to $\pq$. The amount of extra work that is needed to realise the book-keeping necessary for \smart\ (see rows $\textit{RRM1}$, $\textit{RRM2}$, $\textit{RIS}$ and $\textit{RDP}$) is not very significant and seems acceptable given the overall better performance. 
Finally, the alternative prediction means based on BFS are inferior to the machine learning approach, both for $\textsc{bfs}$ and $\textsc{$w$-bfs}$. 

\begin{table*}[ht]
\caption{Average number of various operations of the algorithms and using different prediction algorithms (ML, \textsc{bfs}, \textsc{$w$-bfs}).}
\label{tbl:all_results}
%\vskip 0.15in
\begin{center}
\begin{small}
\begin{sc}
\begin{tabular}{l|r|rrrrrr}
                         & Oracle& Dijks & Prune  & Smart   & Naïve   & bfs & $w$-bfs \\ \hline
$\textit{RM}$                & 59.39        & 59.39 & 59.39        & 59.39   & 152.77  & 59.39      & 59.39                \\
$\textit{IS}$                & 59.39       & 335.50   & 122.91       & 91.73   & 186.53  & 117.66     & 118.86               \\
$\textit{INR}$                & 0.00      & 276.12   & 63.53         & 32.34   & 33.76   & 58.27      & 59.47                \\
$\textit{DP}$                  & 0.78     & 43.96    & 5.87          & 2.89    & 3.37    & 5.29       & 5.46                 \\
$\textit{RRM1}$                      & 0.00     & 0.00    & 0.00      & 0.82    & 0.00    & 0.45       & 0.33                 \\
$\textit{RRM2}$                      & 0.00     & 0.00    & 0.00      & 14.05   & 0.00    & 1.30       & 0.00                 \\
$\textit{RIS}$                      & 0.00     & 0.00    & 0.00      & 46.06   & 0.00    & 7.00       & 4.39                 \\
$\textit{RDP}$                      & 0.00     & 0.00    & 0.00      & 2.16    & 0.00    & 0.14       & 0.08                 \\
$Q$                       & 119.55 & 438.85   & 188.17      & 154.01  & 342.66  & 182.33     & 183.70               \\\hline
%$S$                       & 319.30 & 0.00     & 250.68      & 284.85  & 96.19   & 256.52     & 255.15               \\
%$P$                      & 0.73  & 0.00     & 0.57          & 0.65    & 0.22    & 0.58       & 0.58                 \\\hline
$T$                & 1.00   & 1.00     & 1.00          & 2.28    & 2.28    & 1.23       & 1.00                 \\\hline
$C$                 & 1456.16       & 13949.37 & 5245.96    & 2476.35 & 4973.46 & 4825.09    & 4980.69              \\
$\bar{C}$           & 1.00& 9.58     & 3.60          & 1.70    & 3.42    & 3.31       & 3.42                
\end{tabular}
\end{sc}
\end{small}
\end{center}
\vskip -0.2in
\end{table*}
\fi
